# Supplementary material for: Image Cropping with Composition and Saliency Aware Aesthetic Score Map
Source: arXiv:1911.10492 ancillary file (2019-11-24)
Supplement: Supplementary file 1 [file supplementary.pdf]

# **Supplementary Materials for “Image Cropping with Composition and Saliency Aware Aesthetic Score Map”**

## **Content**

In this file, we demonstrate more image cropping results with 20 images. For each image, we present 7 rectangular cropping results in 7 aspect ratios and 1 circular cropping result.

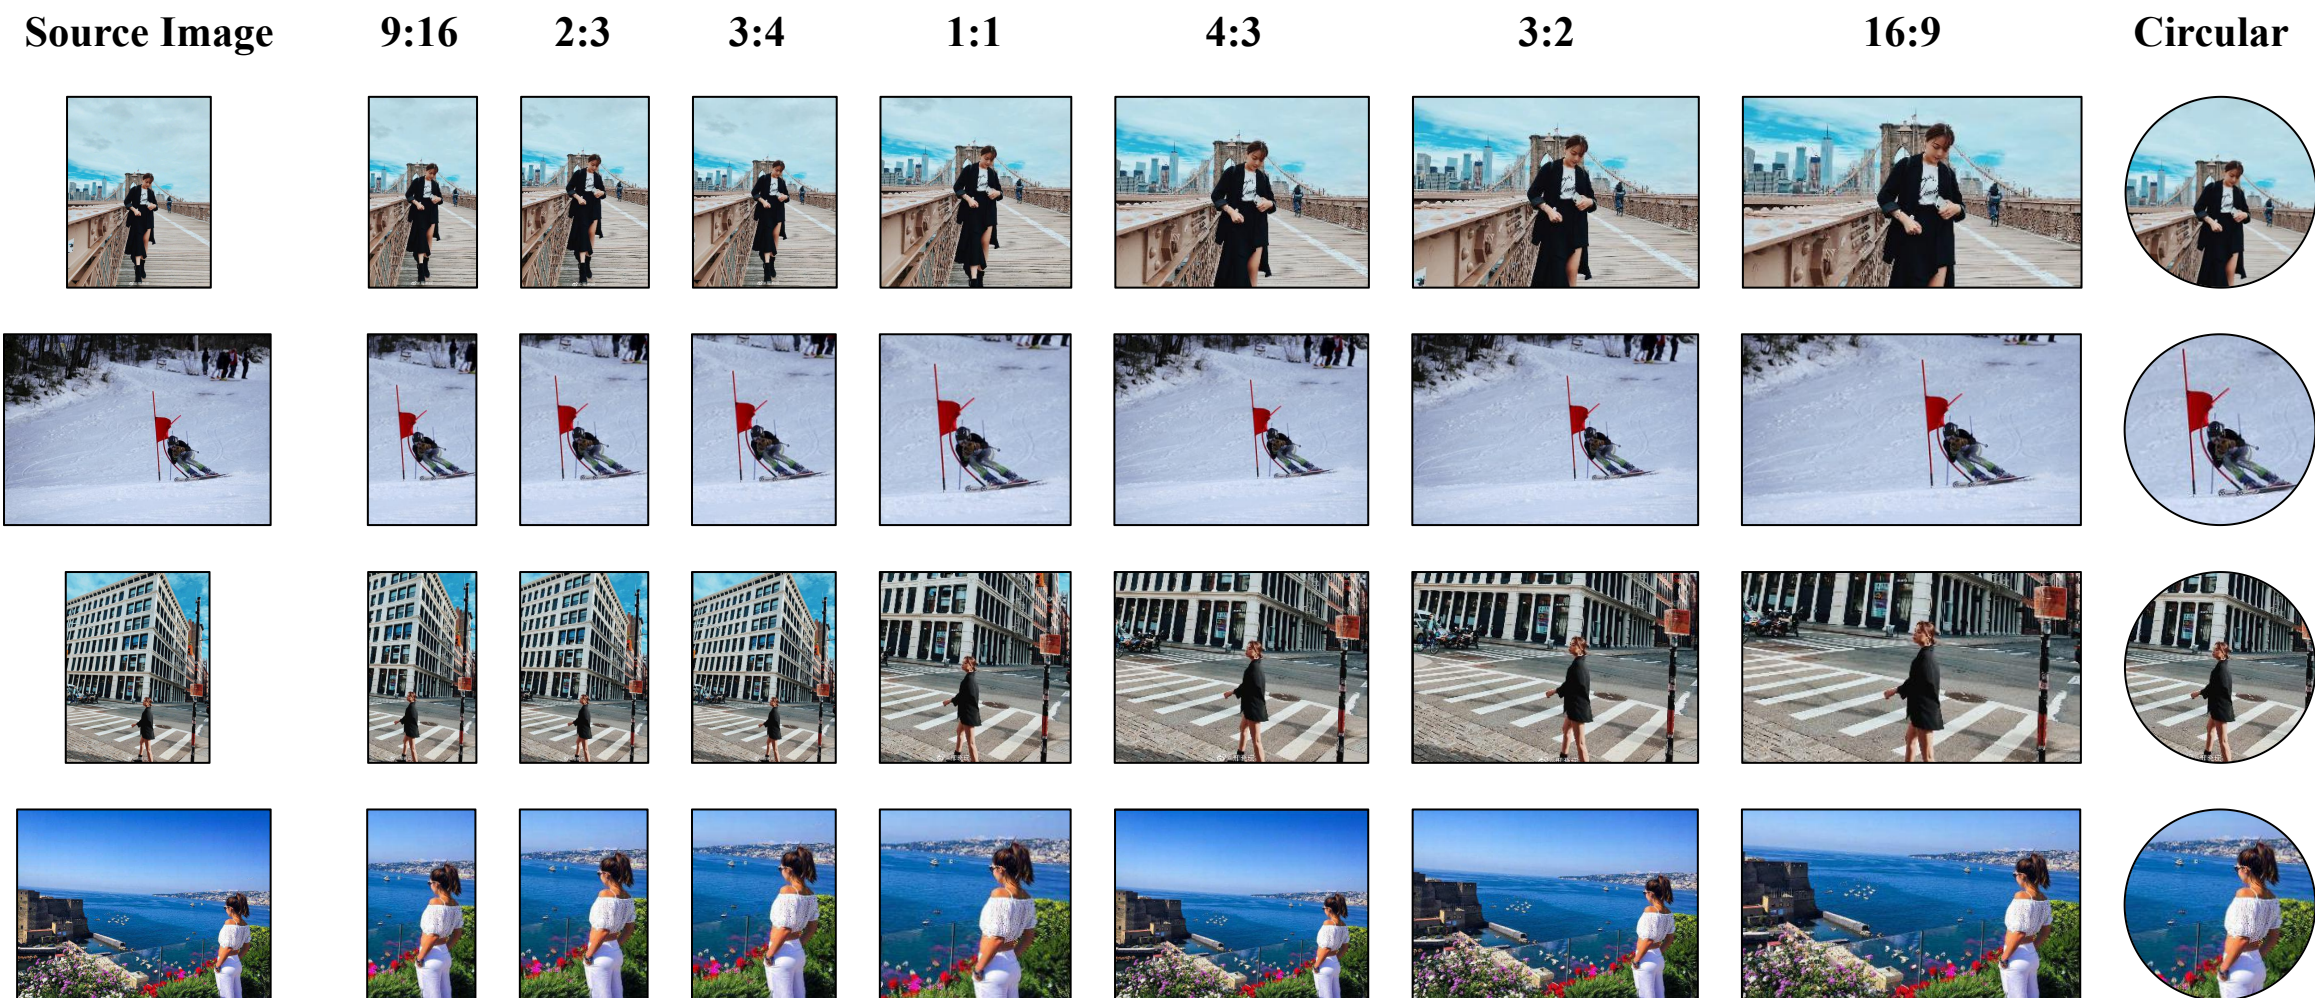

**Figure 1. Photos with a single figure.**



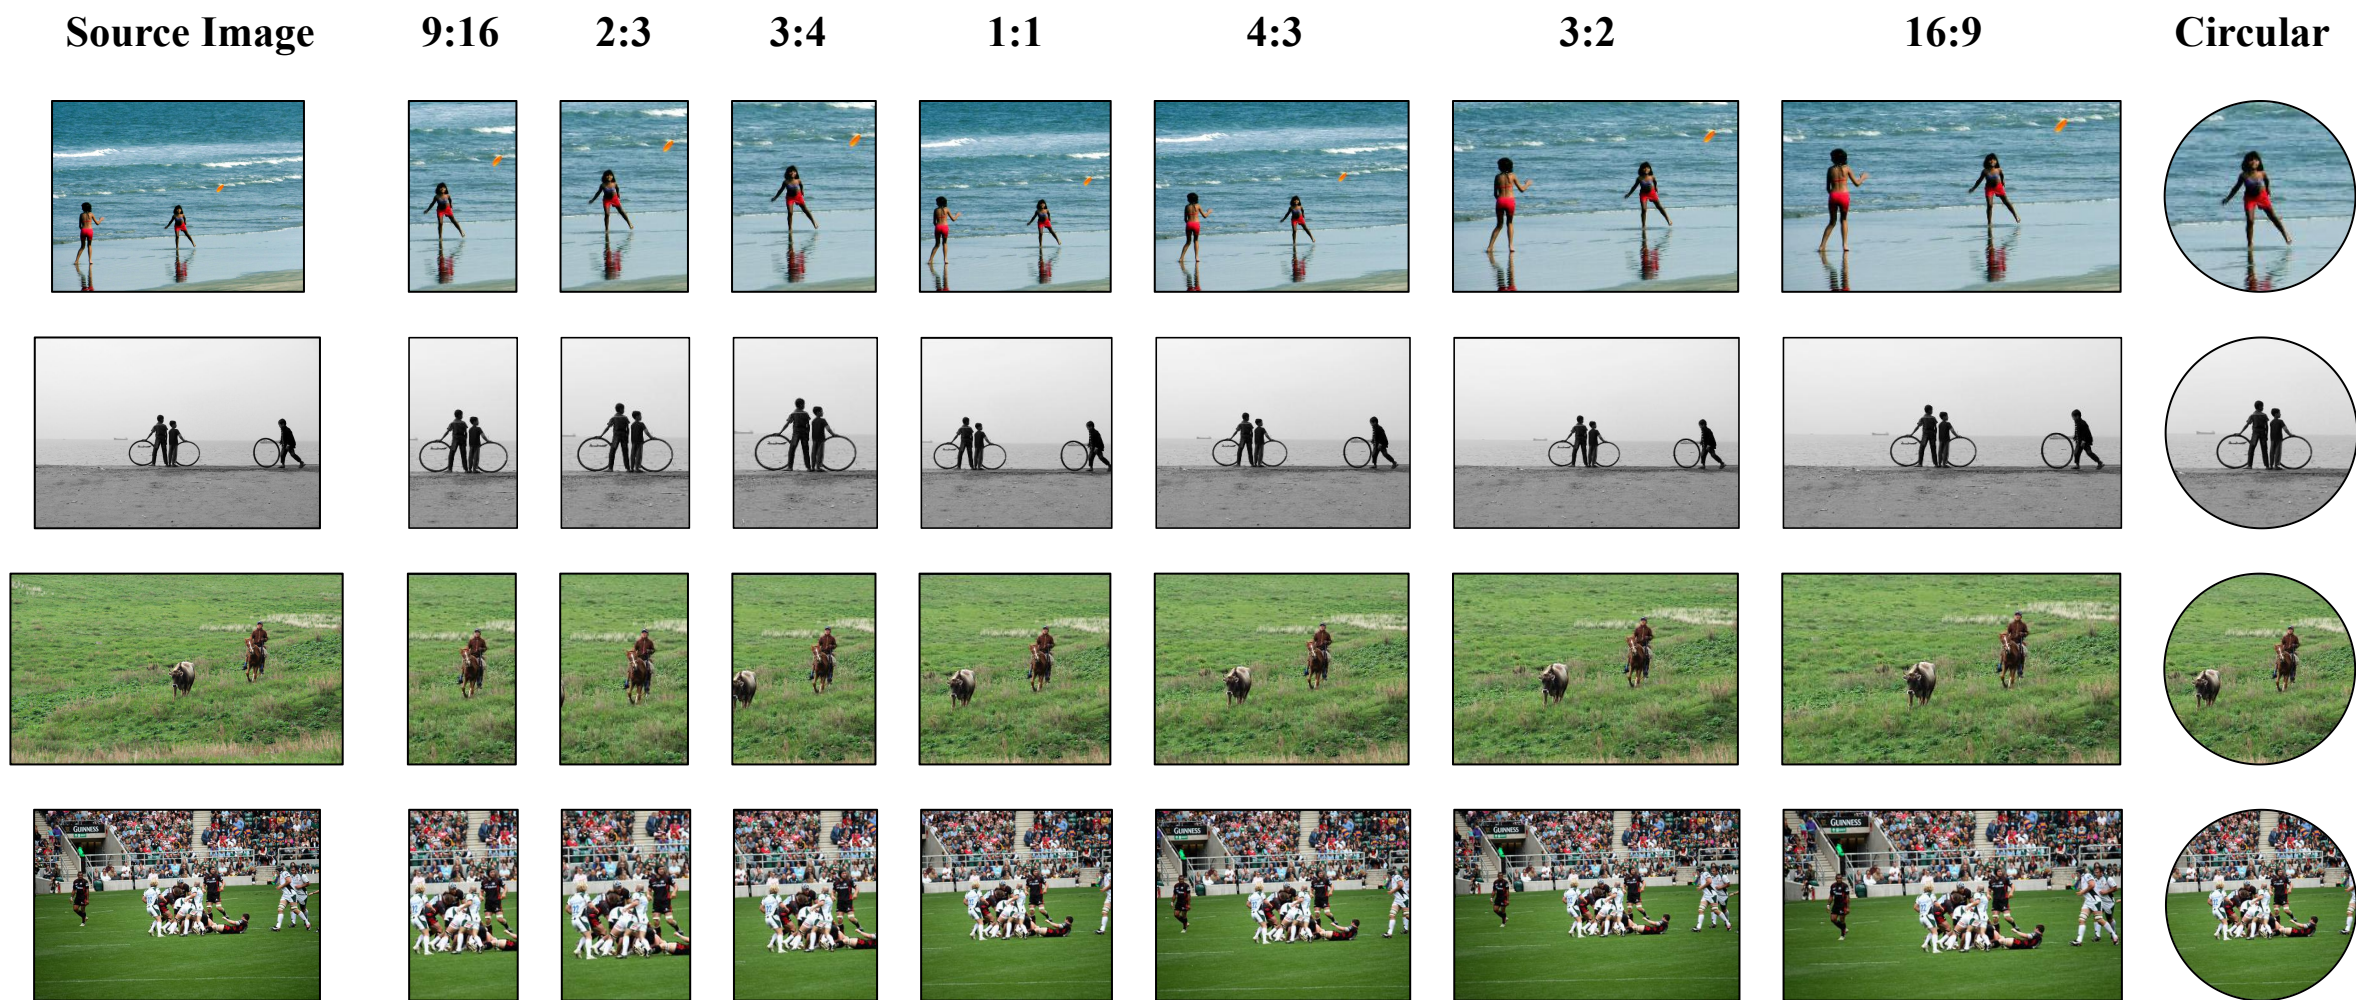

**Figure 2. Photos with multiple figures.**

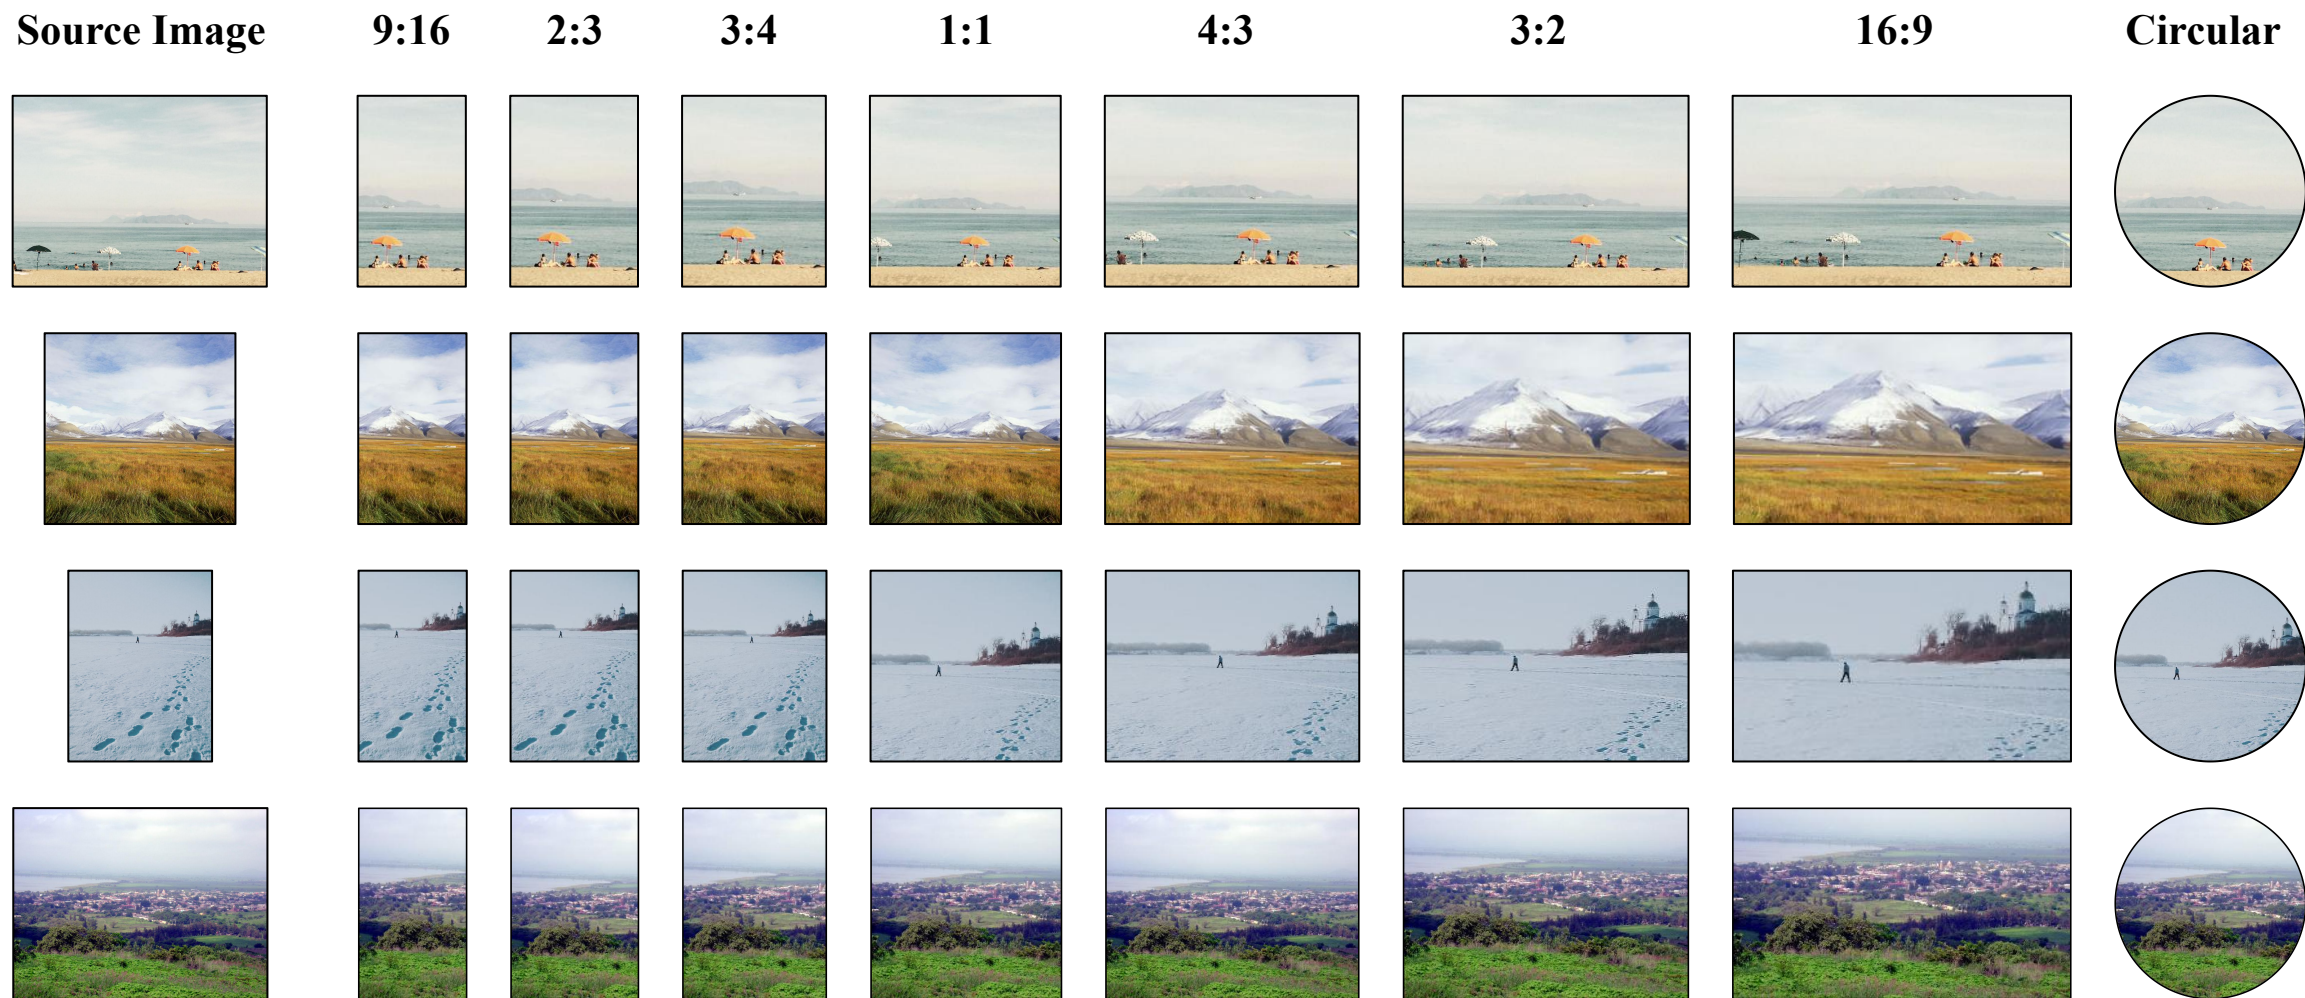

**Figure 3. Landscape photos with no salient object.**



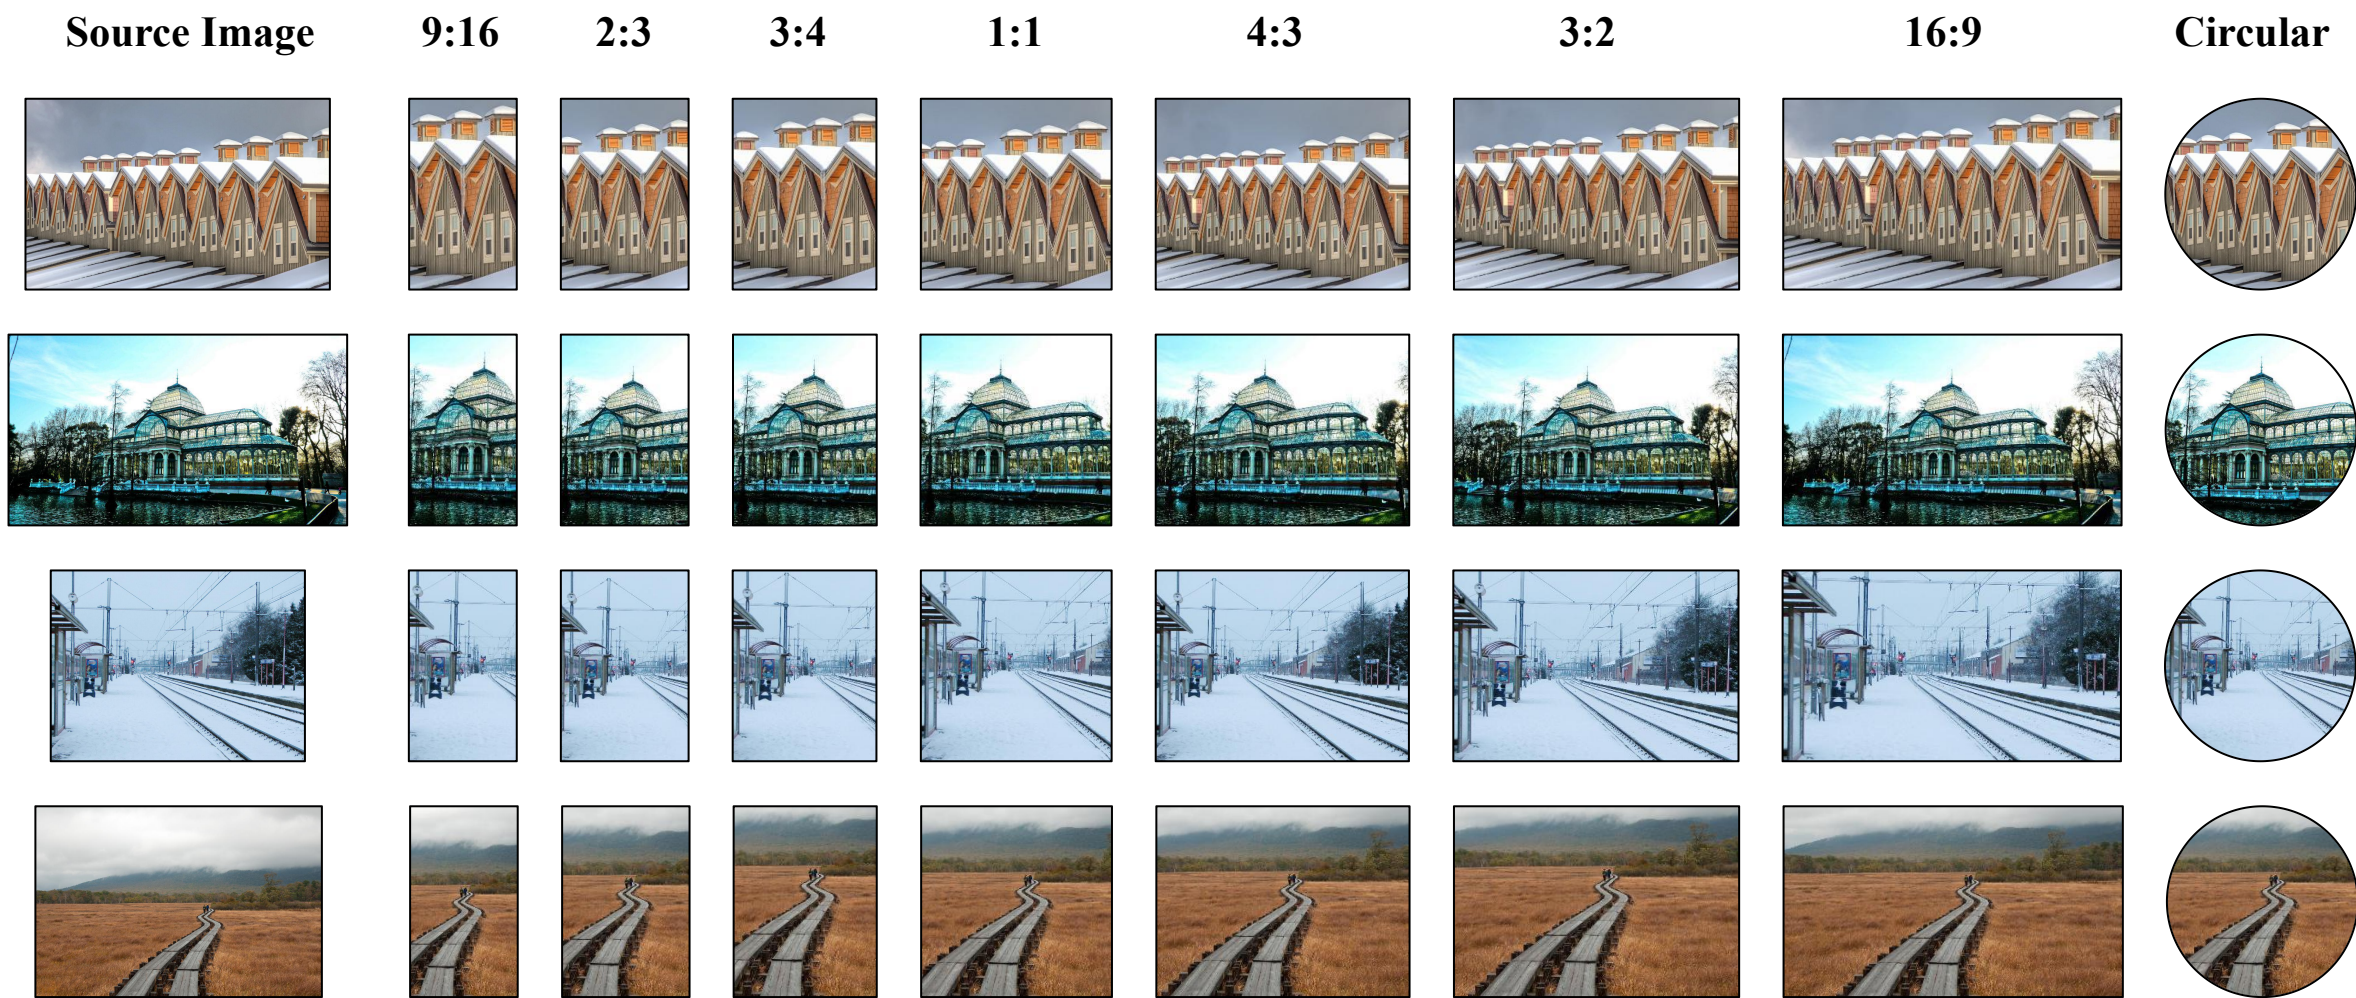

**Figure 4. Photos with architectures or roads.**



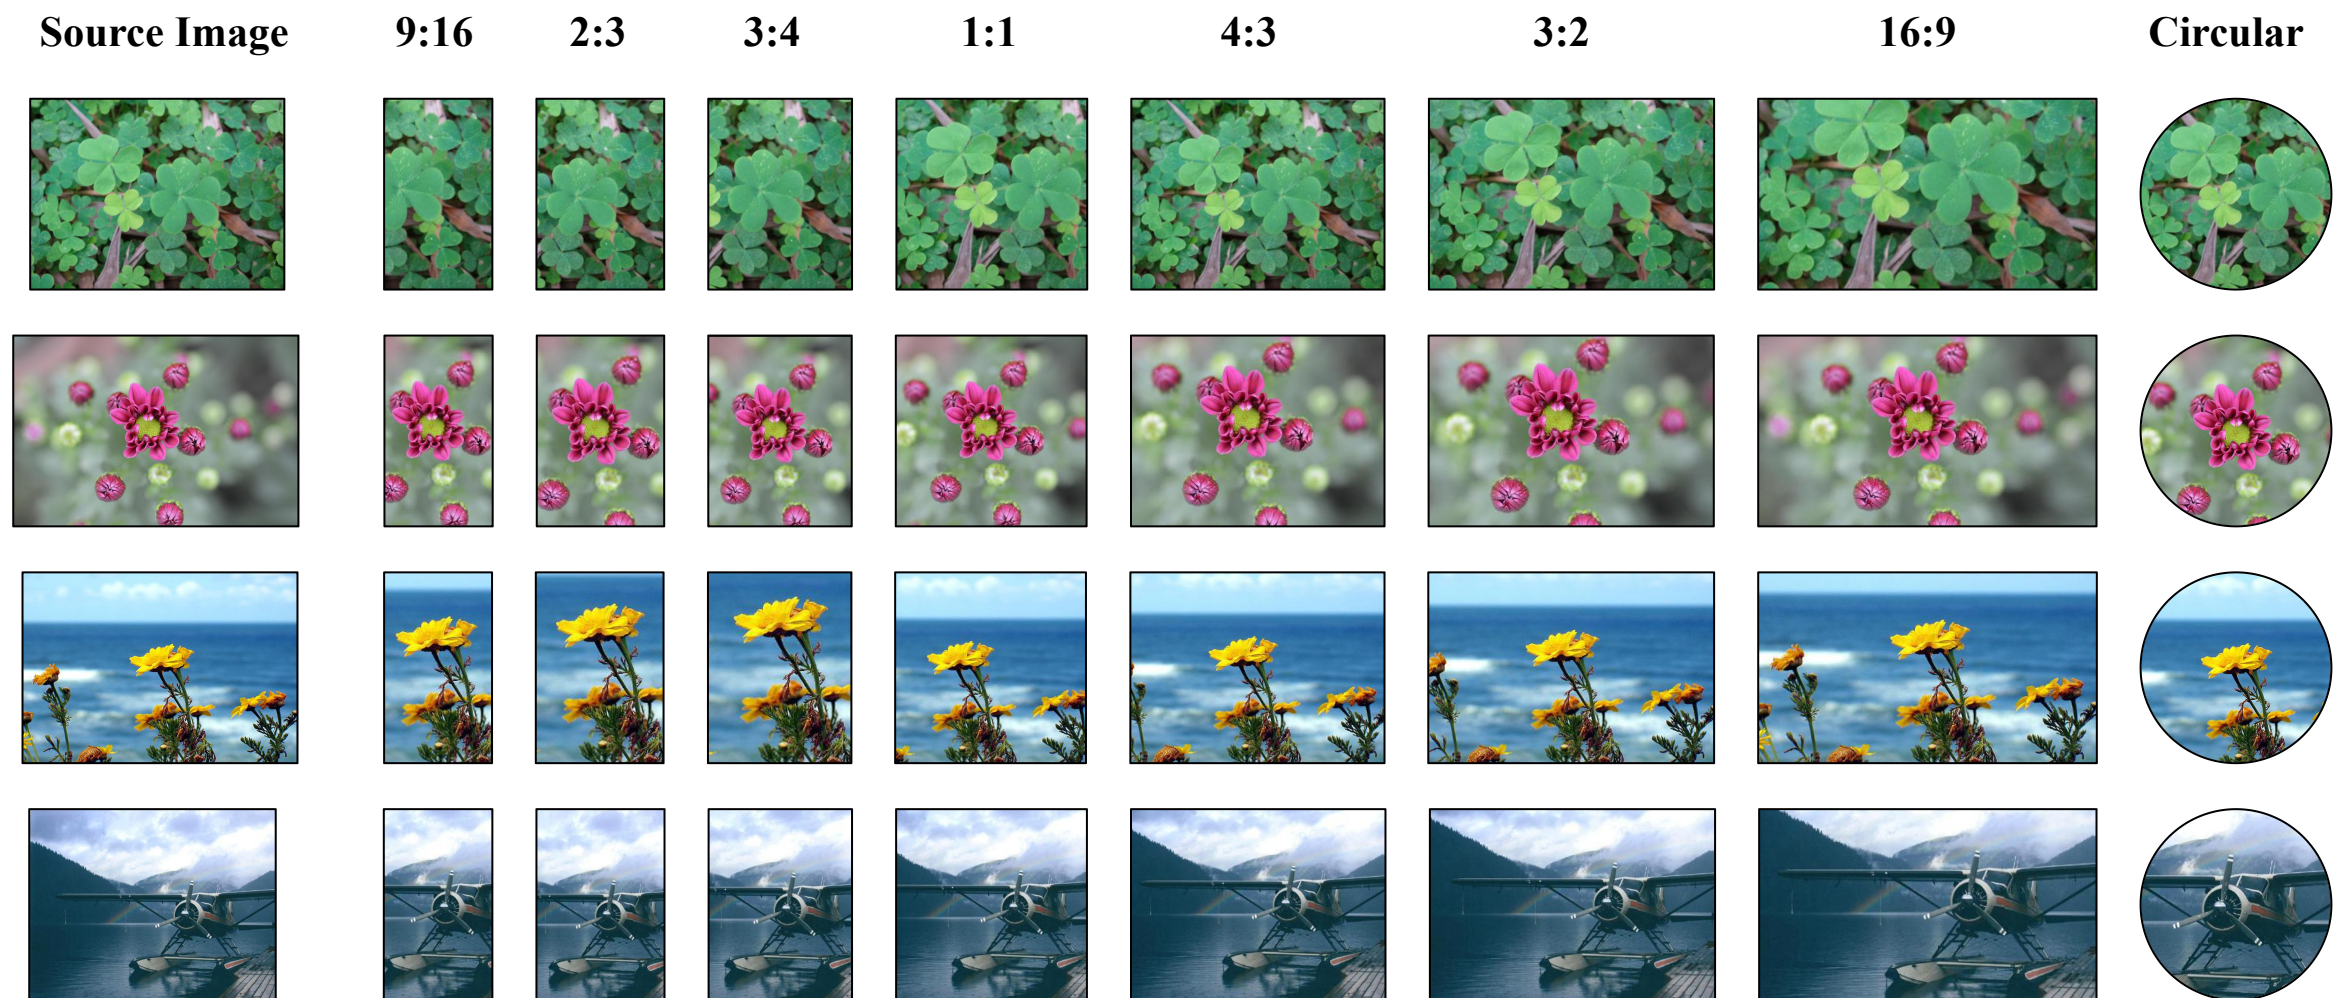

**Figure 5. Photos with complicated background or objects with irregular shapes .**
